# Supplementary material for: Checkpoint-based rollback recovery in session programming
Source: arXiv:2312.02851 source file (2025-01-09)
Supplement: Supplementary file 1 [file multiparty_appendix.tex]

% !TEX root = ../rev_sessions@esop19.tex
\section{Extension to multiparty sessions}
\label{sec:multiparty}

%We discuss in this section 
We show in this Appendix how to extend \cherry, its type discipline,
the compliance checking and the related results, to multiparty 
sessions \cite{KouzapasY14}.

The base sets for the multiparty syntax of \cherry\  are the same
of the binary case, except for \emph{session endpoints}, which now are denoted by 
$s\mendpoint{\role{p}}$, with $\role{p}$,$\role{q}$ ranging over \emph{roles} 
(represented as natural numbers). 
Thus, \emph{session identifiers} $\sessId$ 
now range over session endpoints $s\mendpoint{\role{p}}$ or variables $x$.
The runtime syntax of multiparty \cherry\ is defined by the grammar in 
Fig.~\ref{fig:syntax_cherry_pi_multi}, where expressions $e$ are defined as in the binary case (with values that extends to 
multiparty session endpoints). 
\begin{figure}[t]
\small
	\begin{tabular}{@{}r@{ }c@{\ }l@{\ \ }l@{}}
	$C$ & ::= & $\cdots$    $\mid$ 
	                   $\mrequestAct{a}{\role{p}}{x}{P}$  $\mid$  $\macceptAct{a}{\role{p}}{x}{P}$
	                   & \!\!\!\!\!\!\!\!\!\textbf{Collaborations}
	\\[.3cm]
	$P$ & ::= &  $\cdots$  $\mid$ 
                                        $\msendAct{\sessId}{\role{p}}{e}{P}$ 
		         $\mid$  $\mreceiveAct{\sessId}{\role{p}}{y:S}{P}$ 	
		         $\mid$  $\mselectAct{\sessId}{\role{p}}{l}{P}$ 
		         $\mid$  $\mbranchAct{\sessId}{\role{p}}{\branch{l_1\!\!}{\!\!P_1}
		          \branchSep \ldots \branchSep \branch{l_n\!\!}{\!\!P_n}}$ 
			& \ \ \ \textbf{Processes}
	\\[.1cm]
	\hline
	\end{tabular}
	\vspace*{-.4cm}	
	\caption{Multiparty \cherry\ runtime syntax (the omitted parts are as in Fig.~\ref{fig:syntax_cherry_pi_ext}).}
	%\vspace*{.2cm}	
	\label{fig:syntax_cherry_pi_multi}
\end{figure}
Primitive $\mrequestAct{a}{\role{p}}{x}{P}$ initiates a new session through 
identifier $a$ on the other multiple participants, each one of the form 
$\macceptAct{a}{\role{q}}{x}{P_{\role{q}}}$ where $1 \leq \role{q} \leq \role{p}-1$. 
Variable $x$ will be substituted with the session endpoint used for the interactions
inside the established session. 
Primitive $\msendAct{\sessId}{\role{p}}{e}{P}$ denotes the intention of sending a value to 
role $\role{p}$; similarly, process $\mreceiveAct{\sessId}{\role{p}}{y:S}{P}$ denotes the intention 
of receiving a value from role $\role{p}$. Selection and branching are extended in a similar way.

As usual the operational semantics is given in terms of a structural congruence 
and of a reduction relation. 
The rules defining the structural congruence are standard, while 
%the same ones used for the binary calculus,
%where the rule for the scope extension of session channels takes into account the new form 
%of session endpoints. 
%The reduction relation, instead, is the smallest relation on 
%closed collaborations generated by the rules (an excerpt of which are) reported 
%in Figure~\ref{fig:reduction_pic_multi}.
the forward and backward reduction relations are given by the rules 
in Fig.~\ref{fig:reduction_pic_multi}.
\begin{figure*}[t]
	\centering
	\small
        \begin{tabular}{@{ }c@{}}
	$\msendAct{s\mendpoint{\role{p}}}{\role{q}}{e}{P} 
	\auxrel{\!\send{s\mendpoint{\role{p}}\mendpoint{\role{q}}}{v}\!} \!P$
	\ ($\expreval{e}{v}$)
	 \rulelabel{M-P-Snd}
	\qquad
	$\mreceiveAct{s\mendpoint{\role{p}}}{\role{q}}{y\!:\!S}{P}
	 \auxrel{\!\receive{s\mendpoint{\role{p}}\mendpoint{\role{q}}}{y}\!\!} \!P$
	\rulelabel{M-P-Rcv}
	\\[.5cm]
	\end{tabular}	
	\\
	\begin{tabular}{@{}l@{}}
		$\mrequestAct{a}{n}{x}{P_n}\, \mid \, \prod_{i\in I}\macceptAct{a}{i}{x}{P_i}$ 
	$\ \ \fwred\ \ $
	\\[.1cm]
	\quad 	
	$\singleSession{s\!}{\!(\mrequestAct{a}{n}{x}{P_n}\, \mid \, \prod_{i\in I}\macceptAct{a}{i}{x}{P_i})}$
	\qquad\quad\qquad\qquad\qquad\ \
	$I\!=\!\{1,..,n\!-\!1\}$\quad
	\rulelabel{M-F-Con}	
	\\[.1cm] 	
	\quad 	
        $(\loggedShort{\ce{s}}{P_n\subst{s\mendpoint{n}}{x} }	P_n\subst{s\mendpoint{n}}{x}
        \!\mid\! 
        \prod_{i\in I} \loggedShort{s}{P_i\subst{s\mendpoint{i}}{x}} P_i\subst{s\mendpoint{i}}{x})$
	\\[.5cm]
	\end{tabular}
	\begin{tabular}{@{}c@{}}	
	$
	\infer[$\rulelabel{M-F-Com}$]{
	\loggedShort{\ce{\genSession}}{Q_1} P_1 
	\mid 
	\loggedShort{\genSession}{Q_2} P_2
	\ \fwred\ 
	\loggedShort{\ce{\genSession}}{Q_1} P_1' 
	\mid 
	\loggedShort{\genSession}{Q_2} P_2'\subst{v}{x}	
	}
	{
	P_1 \auxrel{\send{s\mendpoint{\role{p}}\mendpoint{\role{q}}}{v}} P_1'
	& & 
	P_2 \auxrel{\receive{s\mendpoint{\role{q}}\mendpoint{\role{p}}}{x}} P_2'	
	}
	$
	\\[.4cm]
	$
	\infer[$\rulelabel{M-F-Cmt}$]{
	\singleSession{s}{C}(
	\logged{\ce{\genSession}}{Q} P 
	\ \mid \ 
	\prod_{i\in I}\logged{\genSession}{Q_i} P_i)
	\ \fwred\ 
	\singleSession{s}{C}(
	\logged{\ce{\genSession}}{P'} P' 
	\ \mid \ 
	\prod_{i\in I}\logged{\genSession}{P_i} P_i)
	}
	{
	P \auxrel{\commitLab} P'
	}
	$
	\\[.4cm]
	$
	\infer[$\rulelabel{M-B-Rll}$]{
	\singleSession{s}{C}(
	\logged{\ce{\genSession}}{Q} P 
	\ \mid \ 
	\prod_{i\in I}\logged{\genSession}{Q_i} P_i)
	\ \bwred\ 
	\singleSession{s}{C}(
	\logged{\ce{\genSession}}{Q} Q 
	\ \mid \ 
	\prod_{i\in I}\logged{\genSession}{Q_i} Q_i)
	}
	{
	P \auxrel{\rollLab} P'
	}
	$
	\\[.4cm]
	$
	\infer[$\rulelabel{M-B-Abt}$]{
	\singleSession{s}{C}(
	\logged{\ce{\genSession}}{Q} P 
	\ \mid \ 
	\prod_{i\in I}\logged{\genSession}{Q_i} P_i)
	\ \bwred\ 
	C}
	{
	P \auxrel{\abortLab} P'
	}
	$
	\\[.1cm]
	\hline
	\end{tabular}
	\vspace*{-.4cm}	
	\caption{Multiparty \cherry\ semantics: forward and backward reductions (excerpt of rules).}
	\label{fig:reduction_pic_multi}
	\vspace*{.7cm}	
\end{figure*}
%
%The forward and backward reduction relations are given by the rules 
%in Fig.~\ref{fig:reduction_pic_multi}(upper part).
%
We comment on salient points.
Rule \rulelabel{M-F-Con} synchronously initiates a session by requiring all session 
endpoints be present for a forward reduction, where each role $\role{p}$ 
creates a session endpoint $s\mendpoint{\role{p}}$ on a fresh session channel $s$. 
The participant with the maximum role %($\mrequestAct{a}{n}{x}{P_n}$) 
is responsible for requesting a session initiation. Rule \rulelabel{M-F-Com} defines how 
a party with role $\role{p}$ synchronously sends a value to the receiving party with role $\role{q}$. 
Rules \rulelabel{M-F-Cmt}, \rulelabel{M-B-Rll} and \rulelabel{M-B-Abt} are similar to 
those of the binary case, and affect all participants within the considered session. 

The syntax of session types extends to multiparty as shown in Fig.~\ref{fig:typeSyntax_cherry_multi}. 
\begin{figure}[t]
	\centering
	\small
	\begin{tabular}{@{}r@{\ }c@{\ }l@{}l@{}}
	$\typeT\!$ & ::= &  &\!\!  \ldots   $\mid$  
	$\moutType{\role{p}}{\role{q}}{S}.\typeT$  $\,\mid\,$ 
	$\minpType{\role{p}}{\role{q}}{S}.\typeT$   $\,\mid\,$ 
	$\mselType{\role{p}}{\role{q}}{l}.\typeT$ 	$\,\mid\,$  
	$\mbranchType{\role{p}}{\role{q}}{\branch{l_1\!\!}{\!\!\typeT_1}, \ldots, \branch{l_n\!\!}{\!\!\typeT_n}}$
	\ \ \textbf{Types}
	\\[.1cm]
	\hline
	\end{tabular}
	\vspace*{-.6cm}	
	\caption{Multiparty \Cherry\ type syntax 
	(the omitted parts are as in  Fig.~\ref{fig:typeSyntax_cherry_omitted}).
	}
	\label{fig:typeSyntax_cherry_multi}
	%\vspace*{.5cm}
\end{figure}
The session types for output ($\moutType{\role{p}}{\role{q}}{S}.\typeT$)
and input ($\minpType{\role{p}}{\role{q}}{S}.\typeT$) are extended with information 
about the interacting roles; selection and branching types are similarly extended. 
In the type inference, when one of such role is unknown, it is used
a placeholder $\_$ to be filled with a given role; $\typeT\cdot\role{p}$ denotes the type obtained 
from $\typeT$ by filling all its placeholders with the role $\role{p}$.
%
%The \cherry\ type system extends accordingly; as an example we 
%report below the rules for output and input:
%$$
%{\small
%	\infer{\basis;\sorting \judge \msendAct{x}{\role{p}}{e}{P}
%	\hasType x:\moutType{\role{\_}}{\role{p}}{S}.\typeT}
%	{\sorting \judge e \hasType S & & \basis;\sorting \judge P \hasType x:\typeT}
%\qquad\quad
%	\infer{\basis;\sorting \judge \mreceiveAct{x}{\role{p}}{y:S}{P}
%	\hasType x:\minpType{\role{\_}}{\role{p}}{S}.\typeT}
%	{\basis;\sorting\comp y:S \judge P \hasType x:\typeT}
%}
%$$
The \cherry\ type system extends accordingly, as shown in Fig.~\ref{fig:typingSystem_multi}.

% !TEX root = ../rev_sessions@esop19.tex
\begin{figure}[!t]
	\centering
	\small
	\begin{tabular}{c}
	$
	\infer[$\rulelabel{M-T-Req}$]{\mrequestAct{a}{\role{p}}{x}{P} \hasType \{\ce{a}\mendpoint{\role{p}}:\typeT\}}
	{\emptyset;\emptyset \judge P \hasType x:\typeT}
	$		
	\qquad
	$
	\infer[$\rulelabel{M-T-Acc}$]{\macceptAct{a}{\role{p}}{x}{P} \hasType \{a\mendpoint{\role{p}}:\typeT\}}
	{\emptyset;\emptyset \judge P \hasType x:\typeT}
	$
	\\[.4cm]
        $
	\infer[$\rulelabel{M-T-Snd}$]{\basis;\sorting \judge \msendAct{x}{\role{p}}{e}{P}
	\hasType x:\moutType{\role{\_}}{\role{p}}{S}.\typeT}
	{\sorting \judge e \hasType S & & \basis;\sorting \judge P \hasType x:\typeT}
	$
        \\[.4cm]
        $
	\infer[$\rulelabel{M-T-Rcv}$]{\basis;\sorting \judge \mreceiveAct{x}{\role{p}}{y:S}{P}
	\hasType x:\minpType{\role{\_}}{\role{p}}{S}.\typeT}
	{\basis;\sorting\comp y:S \judge P \hasType x:\typeT}
	$
        \\[.4cm]
	$
	\infer[$\rulelabel{M-T-Sel}$]{\basis;\sorting \judge \mselectAct{x}{\role{p}}{l}{P} \hasType 
	x:\mselType{\_}{\role{p}}{l}.\typeT}
	{\basis;\sorting  \judge P \hasType x:\typeT}
	$        
	\\[.4cm]			
	$
	\infer[$\rulelabel{M-T-Br}$]{\basis;\sorting \judge 
	\mbranchAct{x}{\role{p}}{\branch{l_1\!\!}{\!\!P_1}
		          \branchSep \ldots \branchSep \branch{l_n\!\!}{\!\!P_n}}
	\hasType 
	x:\mbranchType{\_}{\role{p}}{\branch{l_1\!\!}{\!\!\typeT_1}, \ldots, \branch{l_n\!\!}{\!\!\typeT_n}}}
	{\basis;\sorting  \judge P_1 \hasType x:\typeT_1 && \ldots 
	 && \basis;\sorting  \judge P_n \hasType x:\typeT_n}
	$
	\\[.1cm]	        
	\hline
	\end{tabular}
	\vspace*{-.3cm}
	\caption{Multiparty \cherry\ typing system (the omitted rules are as in
	Fig.~\ref{fig:typingSystem_coll}, \ref{fig:typingSystem_proc} and \ref{fig:typingSystem_exp_omitted}).}
	%\vspace*{-.1cm}	
	\label{fig:typingSystem_multi}
\end{figure}

The semantics of type configurations is defined only for filled types.
Semantic rules in Fig.~\ref{fig:typeSemantics_ext_multi}
are the natural extension of those for the binary case.
Rule \rulelabel{M-TS-Com} shows that communication affects only 
the two interacting parties, without modifying any checkpoint.
Rule \rulelabel{M-TS-Cmt} sets the checkpoint of the committing party and 
sets an imposed checkpoint for each other party that has performed at least 
an action from its current checkpoint. 
Rule \rulelabel{M-TS-Rll} rolls all parties back to their checkpoints,
provided that the checkpoint of the party requesting the rollback  is not imposed. 
Rule \rulelabel{M-TS-Abt} brings all parties back to the initial configuration.

\begin{figure}[t]
	\centering
	\small
	\begin{tabular}{@{}l@{\qquad\quad}l@{}}
	$\moutType{\role{p}}{\role{q}}{S}.\typeT \typeTrans{\moutType{\role{p}}{\role{q}}{S}} \typeT$\ \ \rulelabel{M-TS-Snd}	
	& 
	$\minpType{\role{p}}{\role{q}}{S}.\typeT \typeTrans{\minpType{\role{p}}{\role{q}}{S}} \typeT$\ \ \rulelabel{M-TS-Rcv}  
	\\[.5cm]
	\multicolumn{2}{@{}c@{}}{
	$
	\infer[$\rulelabel{M-TS-Com}$]
	{\begin{array}{l}
	\minitConf{\typeT^I}
	\conf{\checkpointType{\typeU}_i}{\typeT_i} 
	\confcomp 
	\conf{\checkpointType{\typeU}_j}{\typeT_j}
	\confcomp 	
	\prod_{h\in I-\{i,j\}}\conf{\checkpointType{\typeU}_h}{\typeT_h}
	\\[.1cm] 
	\quad
	\typered
	\ \
	\minitConf{\typeT^I}
	\conf{\checkpointType{\typeU}_i}{\typeT_i'} 
	\confcomp 
	\conf{\checkpointType{\typeU}_j}{\typeT_j'}
	\confcomp 	
	\prod_{h\in I-\{i,j\}}\conf{\checkpointType{\typeU}_h}{\typeT_h}
	\end{array}}
	{\typeT_i \typeTrans{\moutType{\role{p}}{\role{q}}{S}} \typeT_i'
	& &
	 \typeT_j \typeTrans{\minpType{\role{q}}{\role{p}}{S}} \typeT_j'}	
	$
	}
	\\[.8cm]
	\multicolumn{2}{@{}c@{}}{
	$
	\infer[\ \	
	 \checkpointType{\typeU}_h' \! =\!\! 
	 \left\{
	 \begin{array}{ll}
	 \checkpointType{\typeU}_h & \textrm{if}\ \checkpointType{\typeU}_h = \typeT_h \\
	 \imposed{\typeT_h} & \textrm{otherwise}
	 \end{array}
	 \right.
	\ \
	$\rulelabel{M-TS-Cmt}$
	]	
	{
	\begin{array}{l}
	\minitConf{\typeT^I}
	\conf{\checkpointType{\typeU}_i}{\typeT_i} 
	\confcomp 
	\prod_{h\in I-\{i\}}\conf{\checkpointType{\typeU}_h}{\typeT_h}
	\\
	\quad
	\typered
	\ \
	\minitConf{\typeT^I}
	\conf{\typeT_i'}{\typeT_i'} 
	\confcomp 
	\prod_{h\in I-\{i\}}\conf{\checkpointType{\typeU}_h'}{\typeT_h}
	\end{array}
	}
	{\typeT_i \typeTrans{\commitLab} \typeT_i'}	
	$
	}
	\\[.8cm]
	\multicolumn{2}{@{}c@{}}{
	$
	\infer
	{
	\begin{array}{l}
	\minitConf{\typeT^I}
	\conf{\typeU_i}{\typeT_i} 
	\confcomp 
	\prod_{h\in I-\{i\}}\conf{\checkpointType{\typeU}_h}{\typeT_h}
	\
	\typered
	\
	\minitConf{\typeT^I}
	\conf{\typeU_i}{\typeU_i}  
	\confcomp 
	\prod_{h\in I-\{i\}}\conf{\checkpointType{\typeU}_h}{\typeU_h}
	\end{array}
	}
	{\hspace*{4cm}
	\typeT_i \typeTrans{\rollLab} \typeT_i' 
	\hspace*{4cm}
	$\rulelabel{M-TS-Rll}$
	}	
	$
	}
	\\[.8cm]	
	\multicolumn{2}{@{}c@{}}{
	$
	\infer[$\rulelabel{M-TS-Abt}$]
	{
	\begin{array}{l}
	\minitConf{\typeT^I}
	\conf{\checkpointType{\typeU}_i}{\typeT_i} 
	\confcomp 
	\prod_{h\in I-\{i\}}\conf{\checkpointType{\typeU}_h}{\typeT_h}
	\
	\typered
	\
	\minitConf{\typeT^I}
	\prod_{k\in I}\conf{\typeT^k}{\typeT^k}
	\end{array}
	}
	{\typeT_i \typeTrans{\abortLab} \typeT_i' }	
	$	
	}
	\\[.4cm]
	\hline
	\end{tabular}
	\vspace*{-.3cm}	
	\caption{Multiparty \cherry\ type semantics (excerpt of rules, 
	where $I=\{1,\ldots,n\}$, $i,j\in I$, and $\typeT^{I}$ denotes $\typeT^1,\ldots,\typeT^n$).}
	\label{fig:typeSemantics_ext_multi}
	%\vspace*{-.2cm}
\end{figure}

Our notion of \emph{rollback safety}, and the related compliance relation, extend 
to multiparty sessions as follows. Notice that types $\typeT_i$ in 
Def.~\ref{def:rollback_safety_multi} contain placeholders, while in 
Def.~\ref{def:compliance_multi} all types are filled. 

\begin{definition}[Multiparty Rollback safety]\label{def:rollback_safety_multi}
Let $C$ be an initial collaboration, then $C$ is \emph{rollback safe} 
(shortened \emph{\rollSafe}) if $C \hasType \sessions$
and for each $n$-tuple $\ce{a}\mendpoint{\role{n}}:\typeT_n,\ldots,a\mendpoint{\role{1}}:\typeT_1$
in $\sessions$ we have $\compliant(\typeT_n\cdot\role{n},\ldots,\typeT_1\cdot\role{1})$.
\end{definition}

\begin{definition}[Compliance for Multiparty Sessions]\label{def:compliance_multi}
Types $\typeT_1,\ldots,\typeT_n$ are \emph{compliant}, written 
\mbox{$\compliant(\typeT_1,\ldots,\typeT_n)$}, if  
\mbox{$\compliant(\minitConf{\typeT_1,\ldots,\typeT_n}
\conf{\typeT_1}{\typeT_1},\ldots, \conf{\typeT_n}{\typeT_n})$}.
Relation $\compliant$ on type configurations is defined as follows:
$\compliant(\minitConf{\typeT^1,\ldots,\typeT^n}\conf{\checkpointType{\typeU_1}}{\typeT_1},
\ldots,\conf{\checkpointType{\typeU_n}}{\typeT_n})$
holds if for %any
\added{all} $\checkpointType{\typeU}_1'$, $\typeT_1'$, \ldots, $\checkpointType{\typeU}_n'$, $\typeT_n'$ such that
$\minitConf{\typeT^1,\ldots,\typeT^n}
\prod_{h\in \{1,\ldots,n\}}\conf{\checkpointType{\typeU}_h}{\typeT_h}
\typered^*
\minitConf{\typeT^1,\ldots,\typeT^n}
\prod_{h\in \{1,\ldots,n\}}\conf{\checkpointType{\typeU}_h'}{\typeT_h'}
\typered\!\!\!\!\!\!\!\!/\ \ \  $
we have that $\typeT_1'=\ldots=\typeT_n'=\inactType$.
\end{definition}

All notions and concepts of our rollback recovery approach smoothly 
extend to the multiparty case. As consequence, all properties in Sec.~\ref{sec:properties}
still hold in the extended setting; their proofs are in Appendix~\ref{proofs:multiparty}.
% indeed would follow the same structure and only 
%differ for the technicalities concerning the extended definitions. 
We report below just the key theorem concerning session progress.

\begin{theorem}[Multiparty session progress]
\label{th:deadlock_freedom_multi}
Let $C$ be a \rollSafe\ collaboration of the form 
$(\mrequestAct{a}{n}{x}{P_n}\, \mid \, \prod_{i\in \{1,..,n-1\}}\macceptAct{a}{i}{x}{P_i})$.
If $C \fwbwred^* C'$ then either $C' \fwbwred C''$ for some $C''$ or 
$C' \congr \singleSession{s}{C}$ 
$\prod_{i\in \{1,..,n\}}
\logged{{\genSession}}{\checkpointType{Q_i}} \inact\, 
$ for some $\checkpointType{Q_1}, \ldots,\checkpointType{Q_n}$.
\end{theorem}
